# Supplementary material for: Pareto-Optimal Algorithms for Learning in Games
Source: arXiv:2402.09549 source file (2024-02-14)
Supplement: Supplementary file 1 [file appendix_ftl_meanbased.tex]

\section{Mean Based Algorithms and Online Environments}
\label{app:ftl_meanbased}

\esh{We are no longer using this section, but might come in handy for writing the proof of a regret lower bound for FTRL}

We prove some technical properties of mean based algorithms in the general online learning setting. 

We begin by describing the setup -- in each round $i \in [T]$, our algorithm picks an action $a_i$ (possibly using randomness) from a set of experts $A$. After the algorithm makes its choice, the environment reveals a loss $\ell_i(a) \in [-1,1]$ for each action $a$ to the algorithm.

Let $d_t$ denote the historical leader at the start of round $t$, i.e. $d_t \in \argmax_{a \in A} \sum_{i=1}^{t-1
} \ell_i(a)$. The algorithm ``Follow the Leader" (FTL) always plays the historical leader (employing some consistent rule in case of ties) in each round $t \in T$.

Let $\sigma_t^a$ denote the cumulative loss of action $a$ after $t-1$ rounds. 

We recall the definition of mean-based algorithms (from~\cite{deng2019strategizing}), a class of algorithms that generalize FTL, MW and FTPL.

\begin{definition}
    An algorithm is $\gamma$-mean-based if whenever $\sigma_t^a < \sigma_t^j - \gamma T$, the
probability for the algorithm to pick action $a$ on round t is at most $\gamma$. An algorithm is mean-based if it
is $\gamma$-mean-based for some $\gamma$ = o(1).
\end{definition}

We show that FTL cannot do better than the best action in hindsight on any sequence of losses, in other words, FTL has non-negative regret. 

\begin{lemma}  \label{lemma:ftl_positive_regret}
On every loss sequence $\ell$, the loss of FTL, with any tie-breaking rule, is lower bounded by $\min_a \sum_{t=1}^T \ell_t(a) = \sum_{t=1}^T \ell_t(d_{T+1})$.
\end{lemma}

\begin{proof}
Let $d_t$ (the historical leader)  be the action chosen by FTL with an arbitrary tie-breaking rule in round $t$.
    We prove this statement by induction on the total number of rounds $T$. The claim is trivially true for the base case of $T=0$. To extend the hypothesis, assume the statement is true for $T$, i.e., $\sum_{t=1}^T \ell_t(d_t) \ge  \sum_{t=1}^T \ell_t(d_{T+1})$. FTL then plays $d_{T+1}$ in the $t$-round. Adding $\ell_{T+1}(d_{T+1})$ (the loss of FTL in the $T+1$-th round) to both sides of the inequality gives us $\sum_{t=1}^{T+1} \ell_t(d_t) \ge  \sum_{t=1}^{T+1} \ell_t(d_{T+1}) $. However the right hand side is lower bounded by  $\sum_{t=1}^{T+1} \ell_t(d_{T+2})$ since $d_{T+2}$ is the historical leader after $T+1$ rounds. Putting together these inequalities extends the induction hypothesis and proves the lemma.
\end{proof}

Next, we show a useful lemma lower bounding the loss of any mean based algorithm on certain classes of loss sequences. 

We say that the leader $d_t$ after $t-1$ rounds is {\bf $\gamma$-unique} if $\sigma_{t}^{d(t)} < \sigma_t^j - \gamma (t-1)$ for all other actions $j$.

\begin{lemma}
\label{lemma:performance_mb_unique}
    Any $\gamma$ mean-based algorithm $\A$ that acts on a sequence of losses over $T$ rounds such that all but $o(T)$ rounds have a $\gamma$-unique leader has its regret lower bounded by $-(o(T) + 2\gamma T)$. 
\end{lemma}

\begin{proof}
    The proof follows by analyzing the thought experiment that considers the performance of FTL on this loss sequence and compares it to the performance of the particular $\gamma$ mean-based algorithm $\A$. Let the losses be $\ell_1, \ell_2 \cdots \ell_T$. Let FTL (with an arbitrary tie breaking rule) choose some historical leader $d_t$ in round $t$, let $a_t$ denote the action chosen by algorithm $\A$ in round $t$ . Let $I = \{t_1, t_2, \cdots t_k\}$ be the rounds where the algorithm does not have a $\gamma$-unique leader. For all rounds $t \in [T] \setminus I$, there is a $\gamma$-unique leader $d_t$ implying that $a_t = d_t$ with probability at least $1-\gamma$. Thus, the expected loss of $\A$ on any such round can be lower bounded by $(1-\gamma) \ell_t(d_t) - \gamma$ (since the loss of each action is bounded in magnitude by 1). On rounds $t \in I$, the loss of algorithm $\A$ is trivially lower bounded by $-1$. Thus, we get:

    \begin{align*}
        \text{Expected Loss of Algorithm $\A$ } &\ge \sum_{t \in I} -1 + \sum_{t\in [T] \setminus I} ((1-\gamma) \ell_t(d_t) - \gamma) \\
        &\ge -o(T) + \sum_{t\in [T] \setminus I} ((1-\gamma) \ell_t(d_t) - \gamma) \quad \text{ (since $|I| = o(T)$ )}\\
        &\ge -o(T) + \sum_{t \in [T]} \ell_t(d_t) - 2\gamma T \quad \text{( since $\sum_{t \in [T]} |\ell_t(d_t)| \le T$ )} \\
        &\ge -o(T) - 2\gamma T + \min_a \sum_{t=1}^T \ell_t(a) \quad \text{ (applying Lemma~\ref{lemma:ftl_positive_regret} to lower bound $\sum_{t \in [T]} \ell_t(d_t)$)}
    \end{align*}

Comparing the lower bound on the loss to the performance of the single best action in hindsight gives the desired regret lower bound.
\end{proof}
