# Supplementary material for: Pareto-Optimal Algorithms for Learning in Games
Source: arXiv:2402.09549 source file (2024-02-14)
Supplement: Supplementary file 2 [file appendix_mwu_ftpl.tex]

\section{The MWU Algorithm and FTPL}
\label{app:mwu_ftpl}

\esh{Now that we have FTRL, is this section necessary? Should we still keep an explicit version of MWU perhaps?}\jon{I think we can remove this.}

\begin{algorithm}
\caption{Multiplicative Weights Update (MWU)}
\label{alg:mwu}

\SetAlgoNlRelativeSize{0}
\SetAlgoNlRelativeSize{-1}
\SetAlgoNlRelativeSize{-2}
\SetAlgoNlRelativeSize{-2}

\KwData{Number of actions $n$, learning rate $\eta$, time horizon $T$}
\KwResult{Action weights $w_i$ for $i = 1, 2, \ldots, n$}

Initialize weights: $w_i^{(1)} = 1$ for $i = 1, 2, \ldots, n$\;

\For{$t = 1$ \KwTo $T$}{
    Choose action $i_t$ based on the distribution: $p_t(i) = \frac{w_i^{(t)}}{\sum_{j=1}^n w_j^{(t)}}$\;
    Observe payoff vector $\mathbf{c}_t = (c_{1,t}, c_{2,t}, \ldots, c_{n,t})$ for each action\;
    Update weights: $w_i^{(t+1)} = w_i^{(t)} \cdot e^{\eta \cdot c_{i,t}}$ for $i = 1, 2, \ldots, n$\;
}
\end{algorithm}

\begin{theorem}
\label{thm:mwu}
    The Multiplicative Weights Update (MWU) algorithm with learning rate $\eta = \sqrt{\frac{\log n}{T}}$ has the magnitude of its regret for any prefix of rounds bounded by $O(\sqrt{T \log n})$. %This algorithm is $\theta(\frac{1}{\sqrt{T}})$- mean based.
\end{theorem}

\esh{Not sure what's causing the weird (mis)aligns}

The upper bound result is one of the first results in regret minimization, an extensive discussion about it can be found in~\cite{cesa2006prediction}. The lower bound result can be found in~\cite{gofer2016lower} and is also discussed in~\cite{blum2018preserving}.

\esh{Sanity check if the uniform distribution suffices...definitely true if we have already written it as an OLO instance}

\begin{algorithm}
\caption{Follow-the-Perturbed-Leader (FTPL) with Uniform Perturbation}
\label{alg:ftpl}

\SetAlgoNlRelativeSize{0}
\SetAlgoNlRelativeSize{-1}
\SetAlgoNlRelativeSize{-2}
\SetAlgoNlRelativeSize{-2}

\KwData{Number of actions $N$, exploration parameter $\epsilon$, time horizon $T$}
\KwResult{Action sequence $i_t$ for $t = 1, 2, \ldots, T$}

% Uncomment the line below if you want to include initialization
%\State Initialize: $p_i^{(1)} = \frac{1}{N}$ for $i = 1, 2, \ldots, N$\;

Initialize cumulative payoff vector: $\mathbf{P}^{(1)} = \mathbf{0}$\;

\For{$t = 1$ \KwTo $T$}{
    Sample uniform noise vector $\boldsymbol{\eta}_t$ from $[-\epsilon, \epsilon]^N$\;
    Update cumulative payoff vector: $\mathbf{Q} = \mathbf{P}^{(t)} + \boldsymbol{\eta}_t$\;
    Choose action $i_t$ based on the argmax operation: $i_t = \arg\max_i Q_i$\;
    Observe payoff vector $\mathbf{c}_t = (c_{1,t}, c_{2,t}, \ldots, c_{N,t})$ and update cumulative payoff as $\mathbf{P}^{(t)} + \mathbf{c}_t$\;
}
\end{algorithm}

\begin{theorem}
\label{thm:ftpl}
    The Follow-the-Perturbed-Leader (FTPL) algorithm with a suitable choice of $\epsilon$ has the magnitude of its regret for any prefix of rounds bounded by $O(\sqrt{T \log n})$.% For this choice of $\epsilon$, this algorithm is $\theta(\frac{1}{\sqrt{T}})$- mean based.
\end{theorem}

The upper bound result is from~\cite{kalai2005efficient}. The lower bound result can be found in~\cite{gofer2016lower} and is also discussed in~\cite{guzman2021best}.
