# Supplementary material for: Pareto-Optimal Algorithms for Learning in Games
Source: arXiv:2402.09549 source file (2024-02-14)
Supplement: Supplementary file 3 [file appendix_optimality.tex]

\section{Tools for Characterizing Pareto-Optimal Menus}

\label{app:optimality}

 \begin{definition}
     Consider some polytope with a set $T$ of extreme points. For any $x \in T$, let $y$ be a neighbor to $x$ if there exists a direction such that $x$ and $y$ are the sole maximizers in $T$. Equivalently, $x,y \in T$ are said to be neighbours if $Conv(x,y)$ is a $1$-face of the polytope.  We use the notation $N(x)$ to denote the set of neighbors of the extreme point $x$.
 \end{definition}
 
 \begin{lemma}
 \label{lem:path}
 Consider some polytope with a set $T$ of extreme points, and some vector $v$. For any $x \in T$, if $<x,v>$ is no larger than $ <p,v>$ for all $p \in N(x)$, then $<x,v>$ is no larger than $<t,v>$ for all $t \in T$. Furthermore, if $<x,v>$ is no smaller than $<p,v>$ for all $p \in N(x)$, then $<x,v>$ is no smaller than $<t,v>$ for all $t \in T$.  
 \end{lemma}

 \begin{proof}
     \esh{A polytope is spanned by the neighbouring edges of any vertex}

     \esh{https://math.stackexchange.com/questions/3807208/how-to-show-that-any-polytope-p-is-spanned-by-the-neighboring-edges-of-any-ver}
 \end{proof}

% \esh{I think this result with the proof below works for non-polytope menus as well}
 \begin{lemma}
 \label{lemma:unique_points_preserved}
     Consider two algorithms $A$ and $B$ that induce %polytope 
     menus $M_A$ and $M_B$ respectively for some leader payoff $\mu_{\mathcal{L}}$ with menu $M_A$ containing an extreme point $X$ that is not a part of $M_B$. Let $C$ be the convex hull of the union of $A$ and $B$. Then, either $X$ is an extreme point of $C$ or $C$ contains two extreme points $X'$ and $Y'$ such that $X' \in M_A \setminus M_B$ and $Y' \in M_B\setminus M_A $ (note that they would automatically be extreme points of $M_A$ and $M_B$ respectively). 
 \end{lemma}  

 \begin{proof}
    Let $T_A$ ($T_B$) denote the set of extreme points of $M_A$ ($M_B$) that are not a point of $M_B$ ($M_A$). Thus, $X \in T_A$. Let $T$ denote the extreme points of $C$. Either $X \in T$ or $X \notin T$. We only need to consider the second case. In this case, $X$ can be written as a convex combination of extreme points of $C$ - let $T' \subset T$ be a minimal set of extreme points of $C$ such that $X$ can be written as a convex combination of points in $T'$. Since $X$ is not an extreme point of $C$, $X \notin T'$.  It suffices to prove that $T' \cap T_A \ne \phi$ and $T' \cap T_B \ne \phi$, since these results would directly imply a point each from $T_A$ and $T_B$ among the extreme points of $C$ (since $T' \subseteq T$). 
   
    First, to show $T' \cap T_A \ne \phi$, we assume otherwise, which would imply that all the points in $T'$ are extreme points of $M_B$ (since each extreme point of $C$ is either an extreme point of $M_A$ or $M_B$ or both). Thus, $X$ can be written as a convex combination of extreme points of $M_B$, implying that $ X \in M_B$, which is a contradiction, therefore invalidating the assumption.

    For the proof of $T' \cap T_B \ne \phi$, we again attempt to find a contradiction by assuming that this is not true. This implies that $X$ can be written as a convex combination of extreme points of $M_A$ excluding $X$ (since $X \notin T'$). This is a contradiction, since we started with $X$ being an extreme point of $M_A$.
 \end{proof}

 \begin{lemma}
 \label{lem:incomp}
     Consider any two algorithms $A$ and $B$ which, on some $\mu_{\mathcal{L}}$, have polytope menus $M_{A}$ and $M_{B}$ with all max and min learner value points shared. If $M_{A}$ and $M_{B}$ differ on at least one extreme point, $A$ and $B$ are incomparable.
 \end{lemma}

 \begin{proof}
 As $M_{A}$ and $M_{B}$ differ on at least one extreme point and they share all their max and min learner valued points, there must be some extreme point in either $M_{A}$ or $M_{B}$ which gets the learner strictly between their max and min value and is not contained within the other menu. w.l.o.g. let $M_{A}$ contain an extreme point of this form.% , and call this extreme point $a^{*}$.

 Let the polytope $C$ be the convex hull of the union of the extreme points of $M_{A}$ and $M_{B}$. Thus, every extreme point in $C$ must be an extreme point of either $M_{A}$ or $M_{B}$. Let us label the extreme points of $C$ according to which menu they were originally from. If the extreme point is an extreme point in $M_{A}$ but not $M_{B}$, color it red. If it is an extreme point of both menus, or just an extreme point of $M_{B}$, color it blue.  

 Combining our assumption about $M_A$ containing a unique extreme point with Lemma~\ref{lemma:unique_points_preserved}, there must be at least one red point in $C$, $a^{*}$. We claim there is a path through neighboring points from $a^{*}$ to a min-valued learner point such that at each step, the $\mu_{\mathcal{L}}$ value strictly decreases. To see this, note that by Lemma~\ref{lem:path}, as long as the current point is not a minimizing point in the $\mu_{\mathcal{L}}$ direction, there is a way to pick a neighboring point with strictly smaller $\mu_{\mathcal{L}}$. Thus if we continue this process until it is impossible to pick a valid neighbor, we have reached a minimizing point, and the path we took from $a^{*}$ to this point always has strictly decreasing $\mu_{\mathcal{L}}$ value. Call this path $\mathcal{P}$.

 Note that all minimizing points are blue, and $a^{*}$ is red. Thus, when walking from $a^{*}$ to any minimizing point through $\mathcal{P}$, there must be some point of the path where we travel from a red point to a neighboring blue point. Let us call the red point here $r^{*}$ and the blue point $b^{*}$. By our construction of $\mathcal{P}$, it must be the case that $r^{*}$ has a strictly higher $\mu_{\mathcal{L}}$ value than $b^{*}$. Furthermore $r^{*}$ and $b^{*}$ are neighboring points where $r^{*}$ is not contained within $M_{B}$ and $b^{*}$ is an extreme point of $M_{B}$. Thus, by lemma~\ref{Abetter}, there are games where $A$ performs better than $B$.

 Now, we must prove there is a game where $M_{B}$ performs better. 

 We claim there is a path in $C$ through neighboring points from $a^{*}$ to a max-valued learner point such that at each step, the $\mu_{\mathcal{L}}$ value strictly increases. We can again use~\ref{lem:path} to prove this. Call this path $\mathcal{P}$.

 Note that all maximizing points are blue, and $a^{*}$ is red. Thus, when walking from $a^{*}$ to any maximizing point through $\mathcal{P}$, there must be some point of the path where we travel from a red point to a neighboring blue point. Let us call the red point here $r^{*}$ and the blue point $b^{*}$. By our construction of $\mathcal{P}$, it must be the case that $r^{*}$ has a strictly lower $\mu_{\mathcal{L}}$ value than $b^{*}$. Furthermore $r^{*}$ and $b^{*}$ are neighboring points where $r^{*}$ is not contained within $M_{B}$ and $b^{*}$ is an extreme point of $M_{B}$.. Thus, by lemma~\ref{Bbetter}, there are games where $B$ performs better than $A$. 

 As $A$ sometimes performs better than $B$ and $B$ sometimes performs better than $A$, the two algorithms are incomparable.

 \end{proof}
