# Supplementary material for: Pareto-Optimal Algorithms for Learning in Games
Source: arXiv:2402.09549 source file (2024-02-14)
Supplement: Supplementary file 6 [file appendix_srmeanbased_old.tex]

\jon{I moved the main content of this proof to Theorem \ref{thm:high-mb-swap-regret}, but it does not account for perturbations. We should extract the relevant bits here re: how the proof works for perturbations and move them to an appendix}

\esh{Need to fix a misfiring boundary macro}



Fix any fixed learner payoff $\mu_L \in \gameset$. As the main ingredient of the proof, we show a sequence of points appear in the menu of every mean based no-regret algorithm for all large time horizons $T$ that approximately obtain the maximin value (upto subconstant factors), and have significant swap regret. Therefore, their limit point, which appears in the asymptotic menu of every mean-based algorithm; will have exactly the maximin value as well as significant swap-regret, proving
the result.

\begin{claim}
    There is a unique, minimax strategy $M$ against the learner payoff $\mu_L$ with $M$ picking action $X$ with probability $p^* = (2/3 \pm O(\varepsilon)) $ 
\end{claim}
\begin{proof}
    First, we claim that the minmax strategy must cause the learner to be indifferent between at least two of their actions. To see this, assume for contradiction the following cases:

    \begin{itemize}
    \item The minmax strategy $s$ strictly incentivizes $A$ over $B$ and $C$ by $\delta$. Then the optimizer can define a new strategy $(1 - \frac{\delta'}{2})s + \frac{\delta'}{2}Y$ for any $\delta' \leq \delta$, which still incentivizes $A$ but gives the learner strictly lower payoff. The only way this would not decrease payoff is if the strategy was already the pure strategy $Y$, but this cannot incentivize $A$. So this derives a contradiction.
    \item  The minmax strategy $s$ strictly incentivizes $B$ over $A$ and $C$ by $\delta$. Then the optimizer can define a new strategy $(1 - \frac{\delta'}{2})s + \frac{\delta'}{2}X$ for any $\delta' \leq \delta$, which still incentivizes $B$ but gives the learner strictly lower payoff. The only way this would not decrease payoff is if the strategy was already the pure strategy $X$, but this cannot incentivize $B$. So this derives a contradiction.
    \item  The minmax strategy $s$ strictly incentivizes $C$ over $A$ and $B$ by $\delta$. Then the optimizer can define a new strategy $(1 - \frac{\delta'}{2})s + \frac{\delta'}{2}X$ for any $\delta' \leq \delta$, which still incentivizes $B$ but gives the learner strictly lower payoff. The only way this would not decrease payoff is if the strategy was already the pure strategy $X$, but this cannot incentivize $C$. So this derives a contradiction.
    \end{itemize}

    Next, note that $A$ and $C$ are equal when $P(X) = p$ for some $p = \frac{1}{2} \pm O(\epsilon)$. Furthermore, when $P(X) = \frac{1}{2} \pm O(\epsilon)$, $B$ is better than both $A$ and $C$. So there cannot be a minimax strategy when $A$ and $C$ are tied best repsonses. Furthermore, note that $B$ and $C$ are equal when $P(X) = q$ for some $q =  \frac{1}{3} \pm O(\epsilon)$. Against this distribution, the learner can play $C$ and get payoff $\frac{1}{2}.\frac{2}{3} - \frac{1}{2}.\left(\frac{1}{3} \pm O(\epsilon)\right) = \frac{1}{6} \pm O(\epsilon)$. This cannot be the minimax strategy, as if the optimizer just plays $X$, the learner will get payoff at most $\epsilon_{1} < \frac{1}{6} \pm O(\epsilon)$.

    Therefore, the only remaining possibility is that the minmax distribution is when $A$ and $B$ are equal. This is a unique distribution, and will be of the form $P(X) = p^*$ for some  $p^* =  \frac{2}{3} \pm O(\epsilon)$

\end{proof}

%\esh{The proof needs to be fixed from this point onwards}

%\esh{Add sublinear offset by initiallly playing Y to go into the C region}

%\esh{The construction of the sequence has to be changed accordingly}
The CSP $P$ of interest in the finite time menu is constructed by the optimizer playing the following three phase sequence - 
\begin{itemize}
    \item For $T^{\frac{1+\boundary}{2}}$ rounds, play the action $Y$.
    \item For the next $T_1 \sim T/2$ rounds, play the distribution with $P(X) = q$ that has B and C tied as a best response.
    \item For the remaining $T_2 \sim T/2$ rounds, play action $X$.
\end{itemize}
%play a distribution $M'$ for the first $T/2$ rounds and the action $X$ for the remaining $T/2$ rounds. $M'$ is picked so that $M = 1/2 M' + 1/2 X$, i.e. we pick $M'$ such that the time average distribution of the optimizer is exactly equal to the maximin distribution $M$.

We pick $T_1$ so that the resulting marginal distribution of the optimizer over the entire sequence plays action $X$ with probability $p^*$ (i.e. the minimax distribution). This can be done simply by solving a linear equation in one variable. It is not hard to see that $T_1 = (1/2 \pm O(\varepsilon)) T$ and $T_2 = (1/2 \pm O(\varepsilon)) T$.







\begin{claim}
    The learner value of the CSP $P$ is approximately equal to the  $v + \left(\frac{o(T)}{T}\right)$ where $v$ is the maximin value.
\end{claim}

\begin{proof}
     The key observation to make is that the trajectory associated with point $P$ has a $\gamma$-clear leader in all but $o(T)$ time steps. The first phase can be ignored since it is of sublinear length. Since $C$ is a unique best response to $Y$ (by at least $1/12$), $C$ is a $\gamma$-unique  leader at the start of the second phase. The optimizer distribution in each round of the second phase has $B$ and $C$ tied as a best response with both of them being better than $A$ by at least $1/12$. Thus, $C$ remains a $\gamma$-unique leader throughout the second phase. Against optimizer action $X$, $A$ is better than $B$ by at least $1/12$ and $B$ is better than $B$ by at least $1/12$. Thus, over the third phase, the $\gamma$- unique leader turns over from $C$ to $B$ (with a $O(\boundary$) length transition period and since the third phase ends with a tie between $A$ and $B$ for the leader (due to the net marginal distribution being the minimax distribution); $B$ remains a $\gamma$-unique leader except for the last $O(\boundary)$ rounds ~\esh{have to fix some macros here}. 

     Additionally, the marginal distribution of the optimizer over the entire sequence is the minimax distribution implying that the best response to this distribution equals the minimax value. Thus, we conclude using Lemma~\ref{lemma:performance_mb_unique} that the payoff of any mean based learner is approximately equal to the minimax value (upto subconstant factors). The last step of the proof replaces the minimax value with the maximin value (both defined wrt the learner payoff), using Von Neumann's minimax theorem.
\end{proof}


\esh{This is  a bare bones proof, the obervations below can be expanded upon}


Tracking the historical leader over this process allows us to use the mean based property to conclude that:

\begin{itemize}
    \item The time average marginal distribution of the learner in the second phase is almost equal to the pure action $C$ (upto a sub-constant additive  factor).
    \item Studying the time average marginal distribution of the learner in the third phase, the distribution picks action $B$ with $\Omega(1)$, i.e. constant, probability, that is at least $\frac{1}{10}$.  
\end{itemize}

%We also note that all but $o(T)$ rounds has a ``well separated" leader. 

\begin{claim}
    The CSP $P$ has significant swap regret (at least $\frac{1}{360}$).
\end{claim}

\begin{proof}
    The swap function used to demonstrate this swaps action $B$ with action $A$, since $A$ is a better response to $X$ than $B$ with the difference being at least $1/12$. We ignore the sublinear length first phase, and in the second phase $B$ is only played with sub-constant probability, which can again be ignored. However, $B$ is played with marginal probability $\frac{1}{10}$ for $(1/2 \pm O(\varepsilon)) T$ rounds (in the third phase), implying the result.
\end{proof}



To finish the proof, we extend the same arguments to any asymptotic menu. For each time horizon in the corresponding subsequence, we write down the point generated using the above method and conclude that this subsequence of points also converges (since they are identical upto $O(1/T^{\alpha})$ shifts for some $\alpha > 0$. Further, we can use the linearity of payoffs and swap regret against a fixed swap function ,which is switching action $B$ with action $A$, (and hence the continuity) to conclude that the learner payoff of the limit point is exactly the minimax value and that this point has significant swap regret.

Finally, we observe that the same properties can be shown to be true for an extreme point of the asymptotic menu. We simply rewrite the above point as a convex combination of $mn+1$ extreme points of the asymptotic menu (using Caratheodory's theorem). All points in the asymptotic menu must have at least the maximin value due to the no-regret property, thus all the extreme points in the support of this convex decomposition have exactly the maximin value. Swap regret against a fixed swap function is linear, so at least one of the extreme points in the support must have large swap regret, finishing the proof.
